# Supplementary material for: A Framework for Transforming Specifications in Reinforcement Learning
Source: arXiv:2111.00272 source file (2022-05-30)
Supplement: Supplementary file 1 [file appendix.tex]

\section{Proof of Theorem~\ref{thm:discount}}

\section{Proof of Theorem~\ref{thm:no_arm}}

\section{Proof of Lemma~\ref{lem:validprob}}

\section{Proof of Theorem~\ref{thm:nopac}}
